# Supplementary material for: emg2pose: A Large and Diverse Benchmark for Surface Electromyographic Hand Pose Estimation
Source: arXiv:2412.02725 source file (2024-12-02)
Supplement: Supplementary file 1 [file checklist_supplementary.tex]

\section*{Checklist}
\label{sec: checklist}

For the checklist, see the main paper submission, where it is included after the references section.

% \begin{enumerate}

% For the checklist, see the main paper submission, where it is included after the references section.

% \item For all authors...
% \begin{enumerate}
%   \item Do the main claims made in the abstract and introduction accurately reflect the paper's contributions and scope?
%     \answerYes{}
%   \item Did you describe the limitations of your work?
%     \answerYes{} See Section 5. %\cref{sec: discussion}.
%   \item Did you discuss any potential negative societal impacts of your work?
%     \answerYes{} See \cref{sec: societal implications}.
%   \item Have you read the ethics review guidelines and ensured that your paper conforms to them?
%     \answerYes{}
% \end{enumerate}

% \item If you are including theoretical results...
% \begin{enumerate}
%   \item Did you state the full set of assumptions of all theoretical results?
%     \answerNA{}
% 	\item Did you include complete proofs of all theoretical results?
%     \answerNA{}
% \end{enumerate}

% \item If you ran experiments (e.g. for benchmarks)...
% \begin{enumerate}
%   \item Did you include the code, data, and instructions needed to reproduce the main experimental results (either in the supplemental material or as a URL)?
%     \answerYes{} Code, data, and instruction for the reviewers are provided in \cref{sec: dataset_instructions}. Additional information about experiments are included in Section 3 and Appendices A to C (with \cref{sec: full datasheet,sec: dataset_app_details} added in this document for convenience).
%   \item Did you specify all the training details (e.g., data splits, hyperparameters, how they were chosen)?
%     \answerYes{} See \cref{sec: emg2pose_benchmark,sec: full datasheet,sec: dataset_app_details,sec: algorithm_details,table:dataset_details,table:stage_dataset_details,table:hyperparameters}.
% 	\item Did you report error bars (e.g., with respect to the random seed after running experiments multiple times)?
%     \answerYes{} For example, see \cref{table:regression_results,table:tracking_results,fig: results stage breakdown}. We include standard deviation and percentile statistics calculated across users, stages. We do not report errors bars due to multiple model random seeds, as we saw very minimal differences.
% 	\item Did you include the total amount of compute and the type of resources used (e.g., type of GPUs, internal cluster, or cloud provider)?
%     \answerYes{} See \cref{sec: baselines}.
% \end{enumerate}

% \item If you are using existing assets (e.g., code, data, models) or curating/releasing new assets...
% \begin{enumerate}
%   \item If your work uses existing assets, did you cite the creators?
%     \answerYes{} See \cref{sec: baselines} for details on existing baselines that we provide and architectures we use. See \cref{sec: dataset,sec: mocap} for details on the Optitrack system used to collect data. See \cref{sec: semg_sensing} for wrist-band details. See \cref{sec: full datasheet} for details including python packages we build on.
%   \item Did you mention the license of the assets?
%     \answerYes{Dataset and code are licensed under a CC-BY-NC-SA 4.0 license, which is listed in \cref{sec: full datasheet} and repository.} 
%   \item Did you include any new assets either in the supplemental material or as a URL?
%     \answerYes{} We provide videos in zip format to reviewers and further instruction regarding how to access the dataset in \cref{sec: dataset_instructions}.
%   \item Did you discuss whether and how consent was obtained from people whose data you're using/curating?
%     \answerYes{} See \cref{sec: full datasheet}.
%   \item Did you discuss whether the data you are using/curating contains personally identifiable information or offensive content?
%     \answerYes{} In \cref{sec: dataset,sec: full datasheet} we discuss how we remove personally identifiable information.
% \end{enumerate}

% \item If you used crowdsourcing or conducted research with human subjects...
% \begin{enumerate}
%   \item Did you include the full text of instructions given to participants and screenshots, if applicable?
%     \answerNo{We provide a detailed description of the experimental instructions and a list of the movements participants were asked to perform (see \cref{sec: full datasheet,sec: dataset_app_details}).} 
%   \item Did you describe any potential participant risks, with links to Institutional Review Board (IRB) approvals, if applicable?
%     \answerYes{We discuss the consenting process in \cref{sec: full datasheet} and the approval of all research under an external IRB} 
%   \item Did you include the estimated hourly wage paid to participants and the total amount spent on participant compensation?
%     \answerNA{We recruited all participants through a third-party vendor that determined their compensation via market rates. We give details in  \cref{sec: full datasheet}.} 
% \end{enumerate}

% \end{enumerate}
